# Supplementary material for: Pruning-as-Search: Efficient Neural Architecture Search via Channel Pruning and Structural Reparameterization
Source: arXiv:2206.01198 source file (2022-06-02)
Supplement: Supplementary file 1 [file appendix.tex]

% \setcounter{section}{0}
% \setcounter{figure}{0}
% \setcounter{equation}{0}
% \makeatletter 
% \renewcommand{\thefigure}{A\@arabic\c@figure}
% \makeatother
% \setcounter{table}{0}
% \renewcommand{\thetable}{A\arabic{table}}
% \renewcommand{\theequation}{S\arabic{equation}}

\section{Appendix}

\subsection{Magnitude Trap} \label{app: small_magenitude}  
Weight or feature magnitude is widely used as the importance evaluation metric in current pruning arts. 
Pruning policy is decided by the  heuristic  that small magnitudes are less important, which is not necessarily optimal. 
Besides, though there are some variants \cite{liu2017learning,guan2020dais} employing sophisticated regularized training techniques, they still suffer from the magnitude heuristic. 
%we discover that possible variants employing sophisticated regularized training techniques will not jump out of magnitude heuristic as well. 
We refer this phenomenon as magnitude trap. 

We take the indicator approach introduced in \cite{liu2017learning} as baseline, where channel importance is measured by the magnitude of $\gamma$ in batch normalization layer, as it is a scaling multiplier along channel dimension. Taking this method as an example, we investigate three kinds of pruning strategies in the following, demonstrating that they still suffer from the magnitude trap (as shown in Tab.~\ref{fig:appendixa}). 
With the indicators, we can prune the model with the following methods: 
%We take the indicator approach introduced in \cite{liu2017learning} as baseline. 
%Channel importance is measured by the magnitude of $\gamma$ in batch normalization layer, as it is a scaling multiplier along channel dimension. 
(i) We can simply decide pruning policy in one-shot by pruning channels with smaller indicators. 
This method is widely employed and usually exhibit better performance than the coarse uniform pruning policy. 
However, there is no optimality guarantee. 
(ii) A naive improvement of (i) is to update the policy iteratively during regularized training. 
We observe that such approach is ineffective because layers with smaller magnitudes receive more penalty, and are not recoverable. 
As a result, layers pruned more at initial will be pruned more and more, and vice versa, leading to a non-recoverable pruning policy with certain accuracy degradation. 
(iii) In order to update pruning policy to reflect importance shifting during pruning and overcome the weakness of (ii), some work \cite{liu2017learning,guan2020dais} equally penalize all indicators to be close to zero. 
But pruning indicators can not be set in a binary format as our DBC layers because they are correlated with model parameters and have certain functionalities in the model. 
Consequently, equal penalization zeros out overmuch information and inevitably destroys model accuracy. % of super-net. 
In addition, pruned channels are still selected by magnitude after equally regularized training, which makes this method indistinguishable from typical magnitude method. 

Our PaS jumps out of magnitude trap because pruning indicators are decoupled from model parameters and can be directly trained in binary format. 
\cite{liu2017learning} uses $\gamma$ in batch normalization layer as the pruning indicators. But as the pruning indicators   correspond to certain specific functions in the neural network, they can not be treated as binary even if STE is employed.  
%Parameters like $\gamma$ in batch normalization layer correspond to certain specific functions in the neural network, thus can not be treated as binary even if STE is employed. 
Different from  \cite{liu2017learning}, 
%In contrast in our PaS, 
the pruning indicators of the DBC layers in  our PaS method are independent from model functions and does not affect regular DNN training. 

\begin{table*}[]
\centering
\caption{We demonstrate policies generated by (i) one-shot magnitude method, (ii) iteratively updated magnitude method and (iii) equal penalty method, in comparison to our PaS method with DBC layers decoupling pruning policy from magnitudes. We show channel configurations ($3\times 3$ CONV only) compressing ResNet50 to 1 GMACs and compressing RepVGG-B1 to about 3 GMACs here. Method (ii) in RepVGG pruning crashes to random guess during updating, we conclude this as falling into a  dead end where inappropriate layers are over-pruned.}
\begin{tabular}{c|ccccc}
\toprule
    ResNet50     & Baseline & One-shot magnitude & Iterative update & Equal penalty & PaS w. DBC \\
\hline
Top-1 (\%) & 77.1     & 73.4               & 54.0             & 72.4          & 74.8       \\
\hline
layer1   & 64       & 58                 & 64               & 38            & 31         \\
layer3   & 64       & 17                 & 0                & 26            & 3          \\
layer6   & 64       & 29                 & 0                & 22            & 3          \\
layer9   & 64       & 59                 & 0                & 25            & 0          \\
layer12  & 128      & 87                 & 61               & 61            & 58         \\
layer15  & 128      & 31                 & 32               & 54            & 30         \\
layer18  & 128      & 66                 & 11               & 83            & 17         \\
layer21  & 128      & 96                 & 9                & 122           & 31         \\
layer24  & 256      & 103                & 248              & 198           & 157        \\
layer27  & 256      & 126                & 225              & 119           & 73         \\
layer30  & 256      & 139                & 247              & 164           & 74         \\
layer33  & 256      & 81                 & 237              & 78            & 44         \\
layer36  & 256      & 106                & 137              & 49            & 38         \\
layer39  & 256      & 151                & 95               & 82            & 22         \\
layer42  & 512      & 353                & 506              & 479           & 440        \\
layer45  & 512      & 468                & 510              & 494           & 445        \\
layer47  & 512      & 452                & 508              & 497           & 475       \\
\bottomrule
\end{tabular}
\begin{tabular}{c|ccccc}
\toprule
RepVGG   & Baseline & One-shot magnitude & Iterative update & Equal penalty & PaS w. DBC \\
\hline
Top-1 (\%) & 78.37    & 72.71              & 0.1                & 72.97         & 75.86      \\
\hline
layer1   & 64       & 42                 & -                & 16            & 32         \\
layer2   & 128      & 94                 & -                & 25            & 43         \\
layer3   & 128      & 108                & -                & 28            & 46         \\
layer4   & 128      & 103                & -                & 23            & 47         \\
layer5   & 128      & 89                 & -                & 20            & 45         \\
layer6   & 256      & 160                & -                & 58            & 127        \\
layer7   & 256      & 101                & -                & 49            & 68         \\
layer8   & 256      & 99                 & -                & 47            & 79         \\
layer9   & 256      & 88                 & -                & 56            & 93         \\
layer10  & 256      & 147                & -                & 68            & 113        \\
layer11  & 256      & 46                 & -                & 68            & 96         \\
layer12  & 512      & 343                & -                & 177           & 269        \\
layer13  & 512      & 229                & -                & 169           & 146        \\
layer14  & 512      & 325                & -                & 165           & 154        \\
layer15  & 512      & 326                & -                & 149           & 141        \\
layer16  & 512      & 283                & -                & 171           & 164        \\
layer17  & 512      & 251                & -                & 204           & 178        \\
layer18  & 512      & 224                & -                & 216           & 171        \\
layer19  & 512      & 212                & -                & 275           & 220        \\
layer20  & 512      & 186                & -                & 304           & 232        \\
layer21  & 512      & 173                & -                & 322           & 236        \\
layer22  & 512      & 166                & -                & 351           & 263        \\
layer23  & 512      & 111                & -                & 376           & 297        \\
layer24  & 512      & 137                & -                & 411           & 360        \\
layer25  & 512      & 273                & -                & 422           & 434        \\
layer26  & 512      & 291                & -                & 434           & 479        \\
layer27  & 512      & 59                 & -                & 414           & 440       \\
\bottomrule
\end{tabular}
\label{fig:appendixa}
\end{table*}

\subsection{More PaS Searched Architectures} \label{app: searched_arch}  

We provide more PaS searched architectures in this section, including pruning ResNet50 and RepVGG-B1 under different pruning targets (Fig.~\ref{fig:appendixb0} and ~\ref{fig:appendixb}), searched channel configurations of YOLACT Fig.~\ref{fig:appendixc}) and GAN models (Fig.~\ref{fig:appendixd}). 
We demonstrate some examples of the image translation on horse to zebra translation benchmark with our PaS model compared to \cite{li2020gan}, based on the CycleGAN ~\cite{zhu2020unpaired} model in Fig.~\ref{fig:appendixe}.

\begin{figure}[]
  \small
  \centering
  \includegraphics[width=0.9\columnwidth]{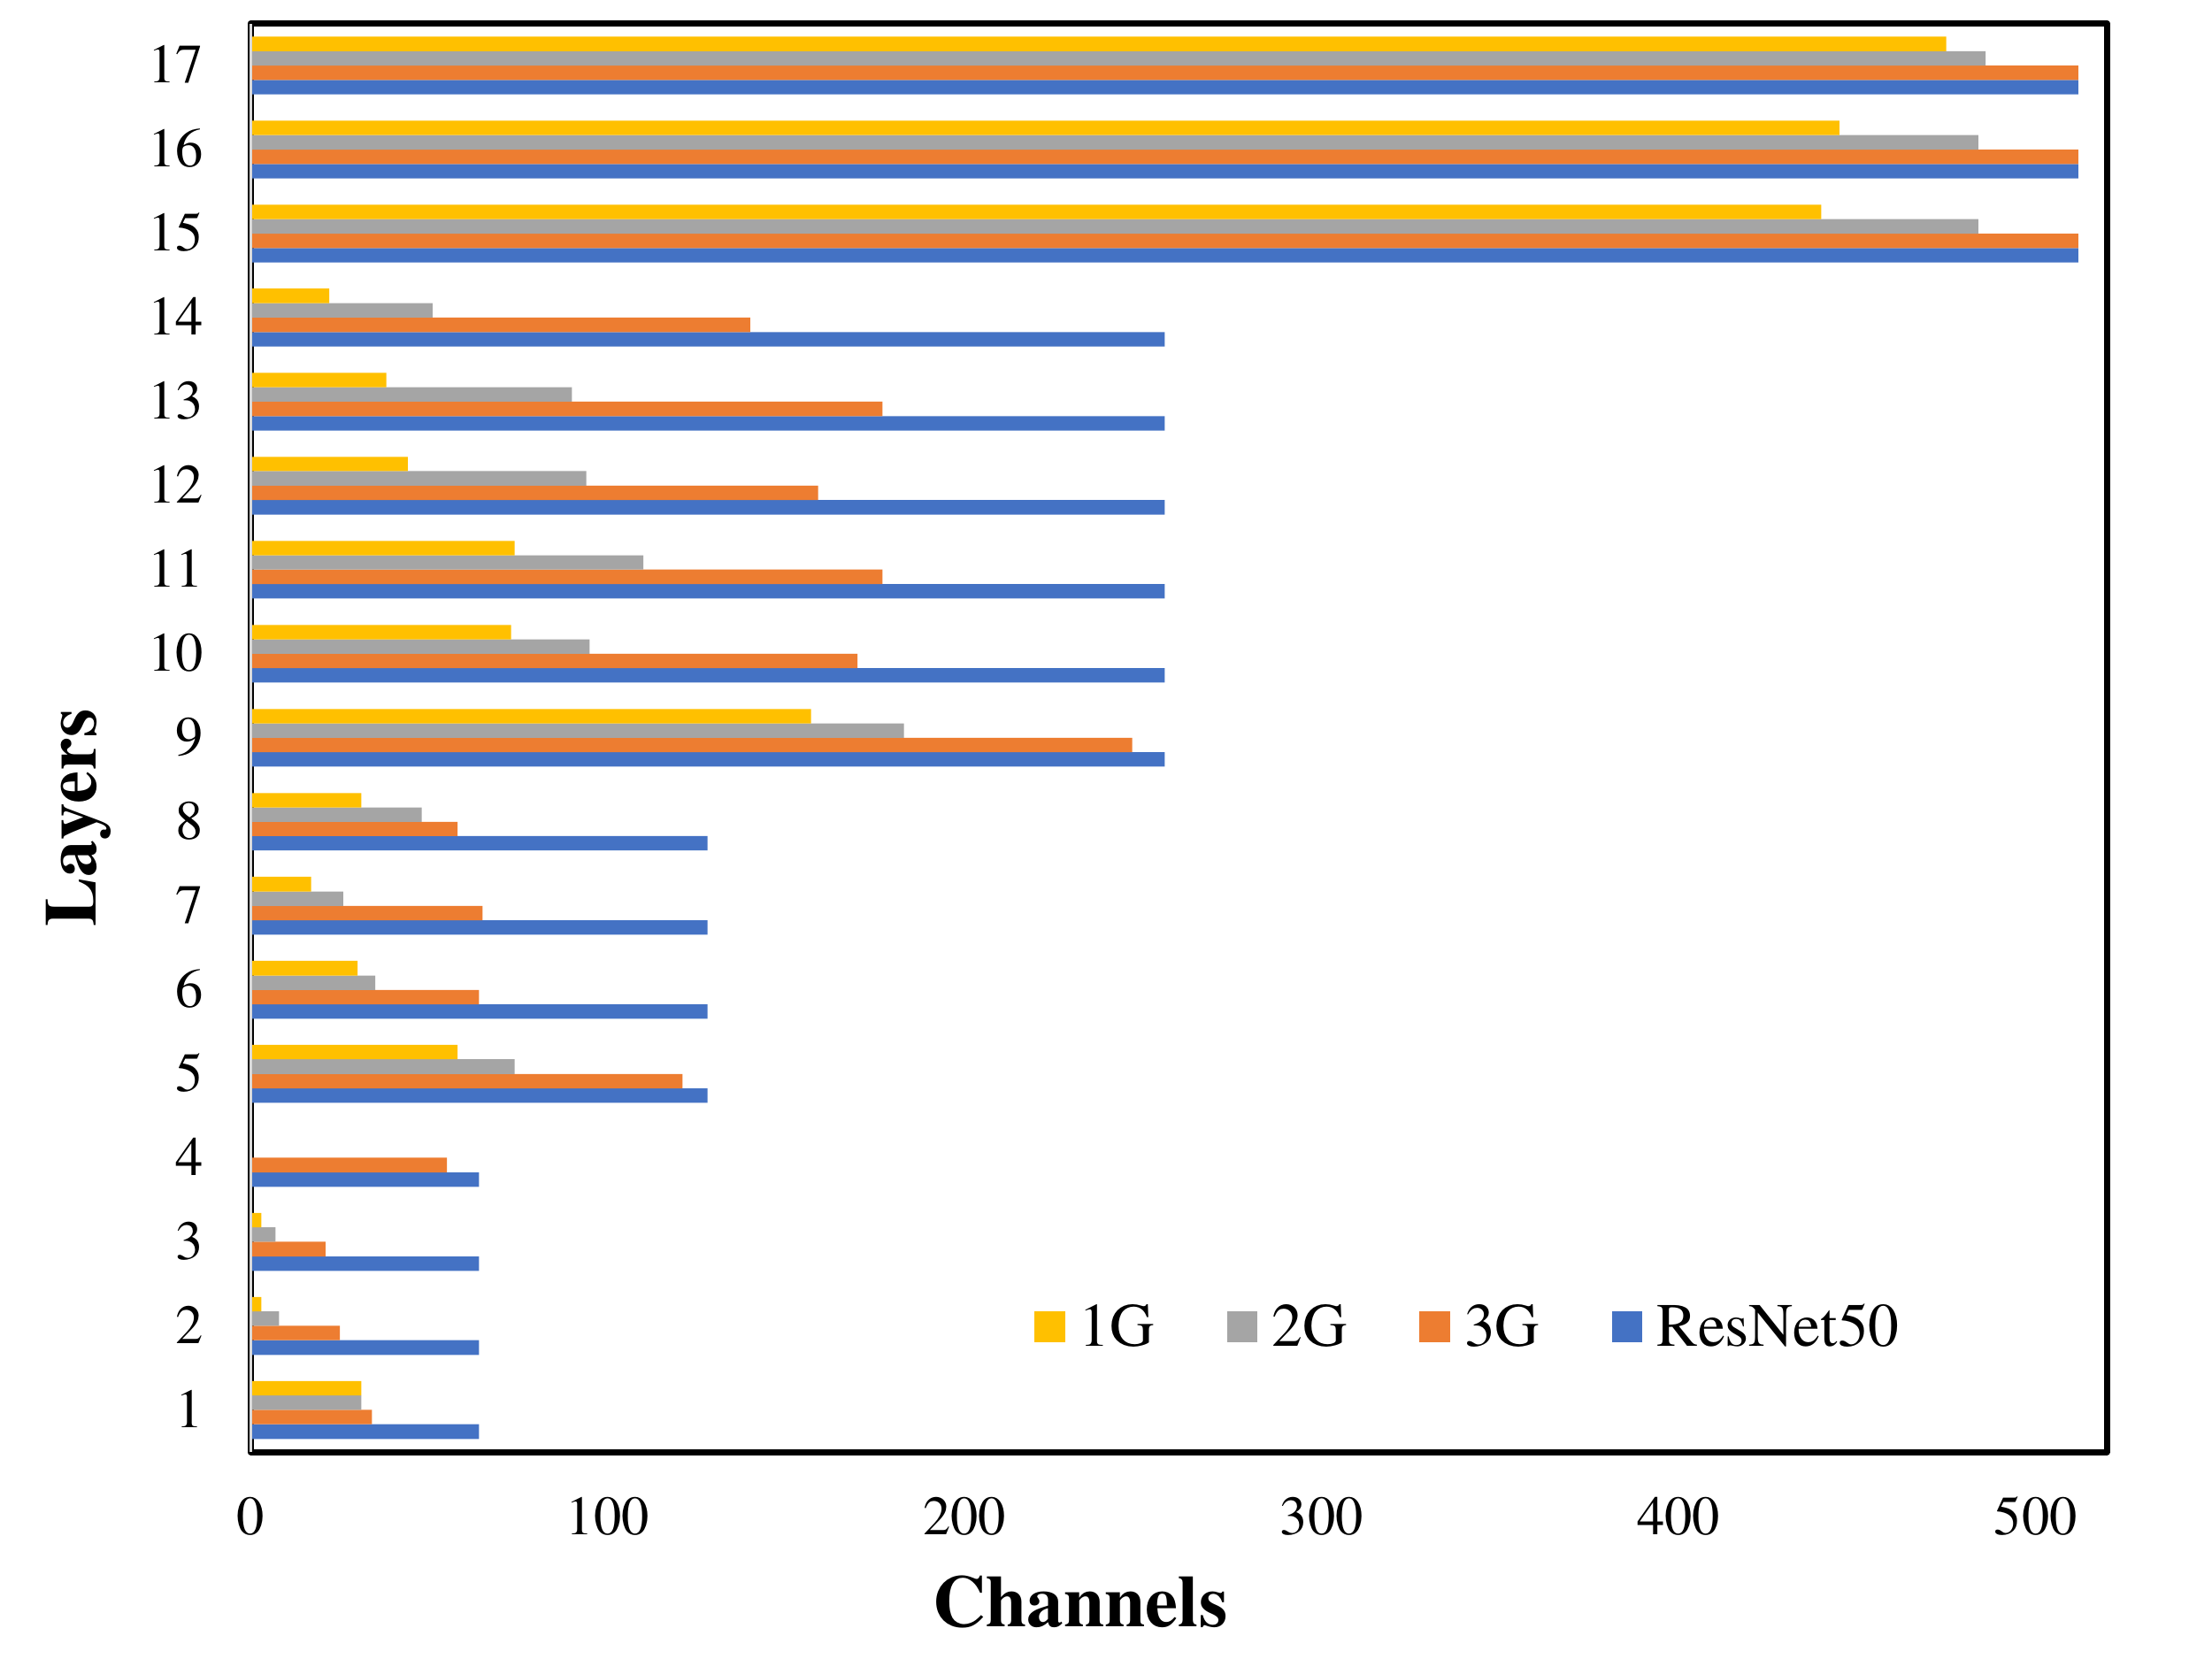}
  \caption{A series of PaS searched channel configurations starting from ResNet50 model with different computation complexity (MACs) targets. We only show $3\times 3$ convolution layers for better visualization. }
  \label{fig:appendixb0}
\end{figure}

\begin{figure}[]
  \small
  \centering
  \includegraphics[width=0.9\columnwidth]{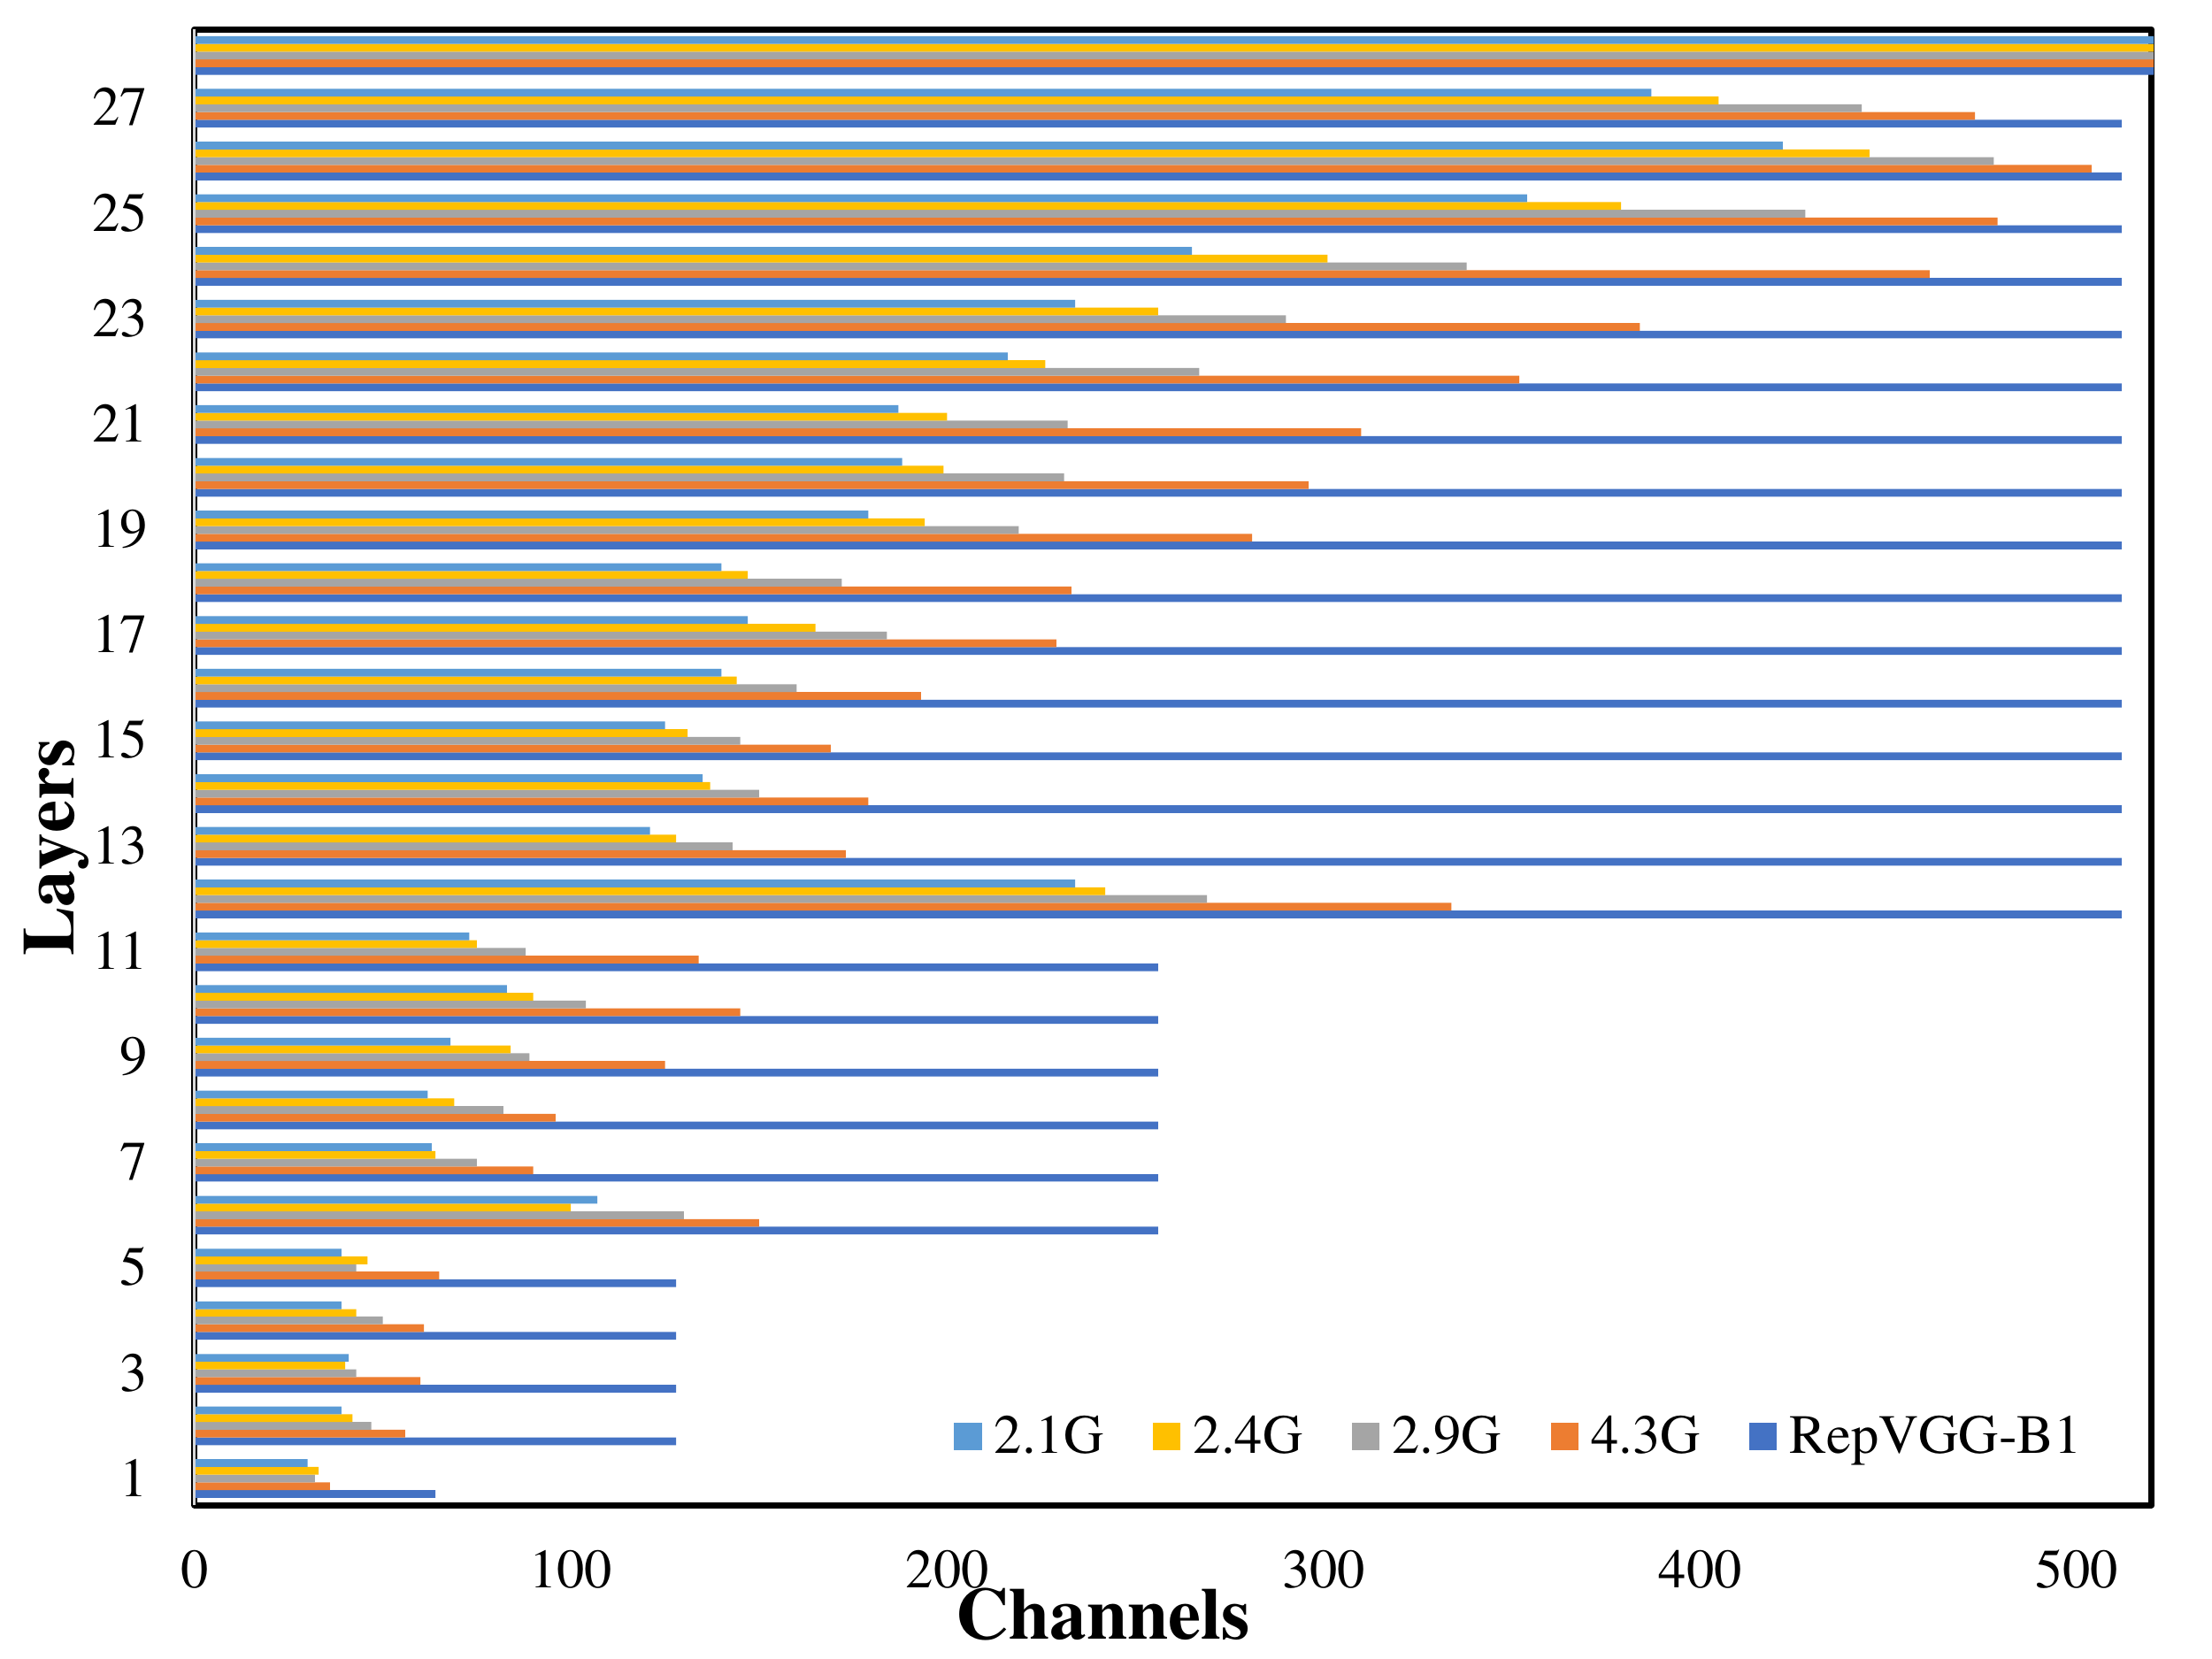}
  \caption{A series of PaS searched channel configurations starting from RepVGG-B1 model with different computation complexity (MACs) targets. For better visualization, the last convolution layer (layer-28) is not presented as it generally remains full width (2048). }
  \label{fig:appendixb}
\end{figure}

\begin{figure}[]
  \small
  \centering
  \includegraphics[width=0.9\columnwidth]{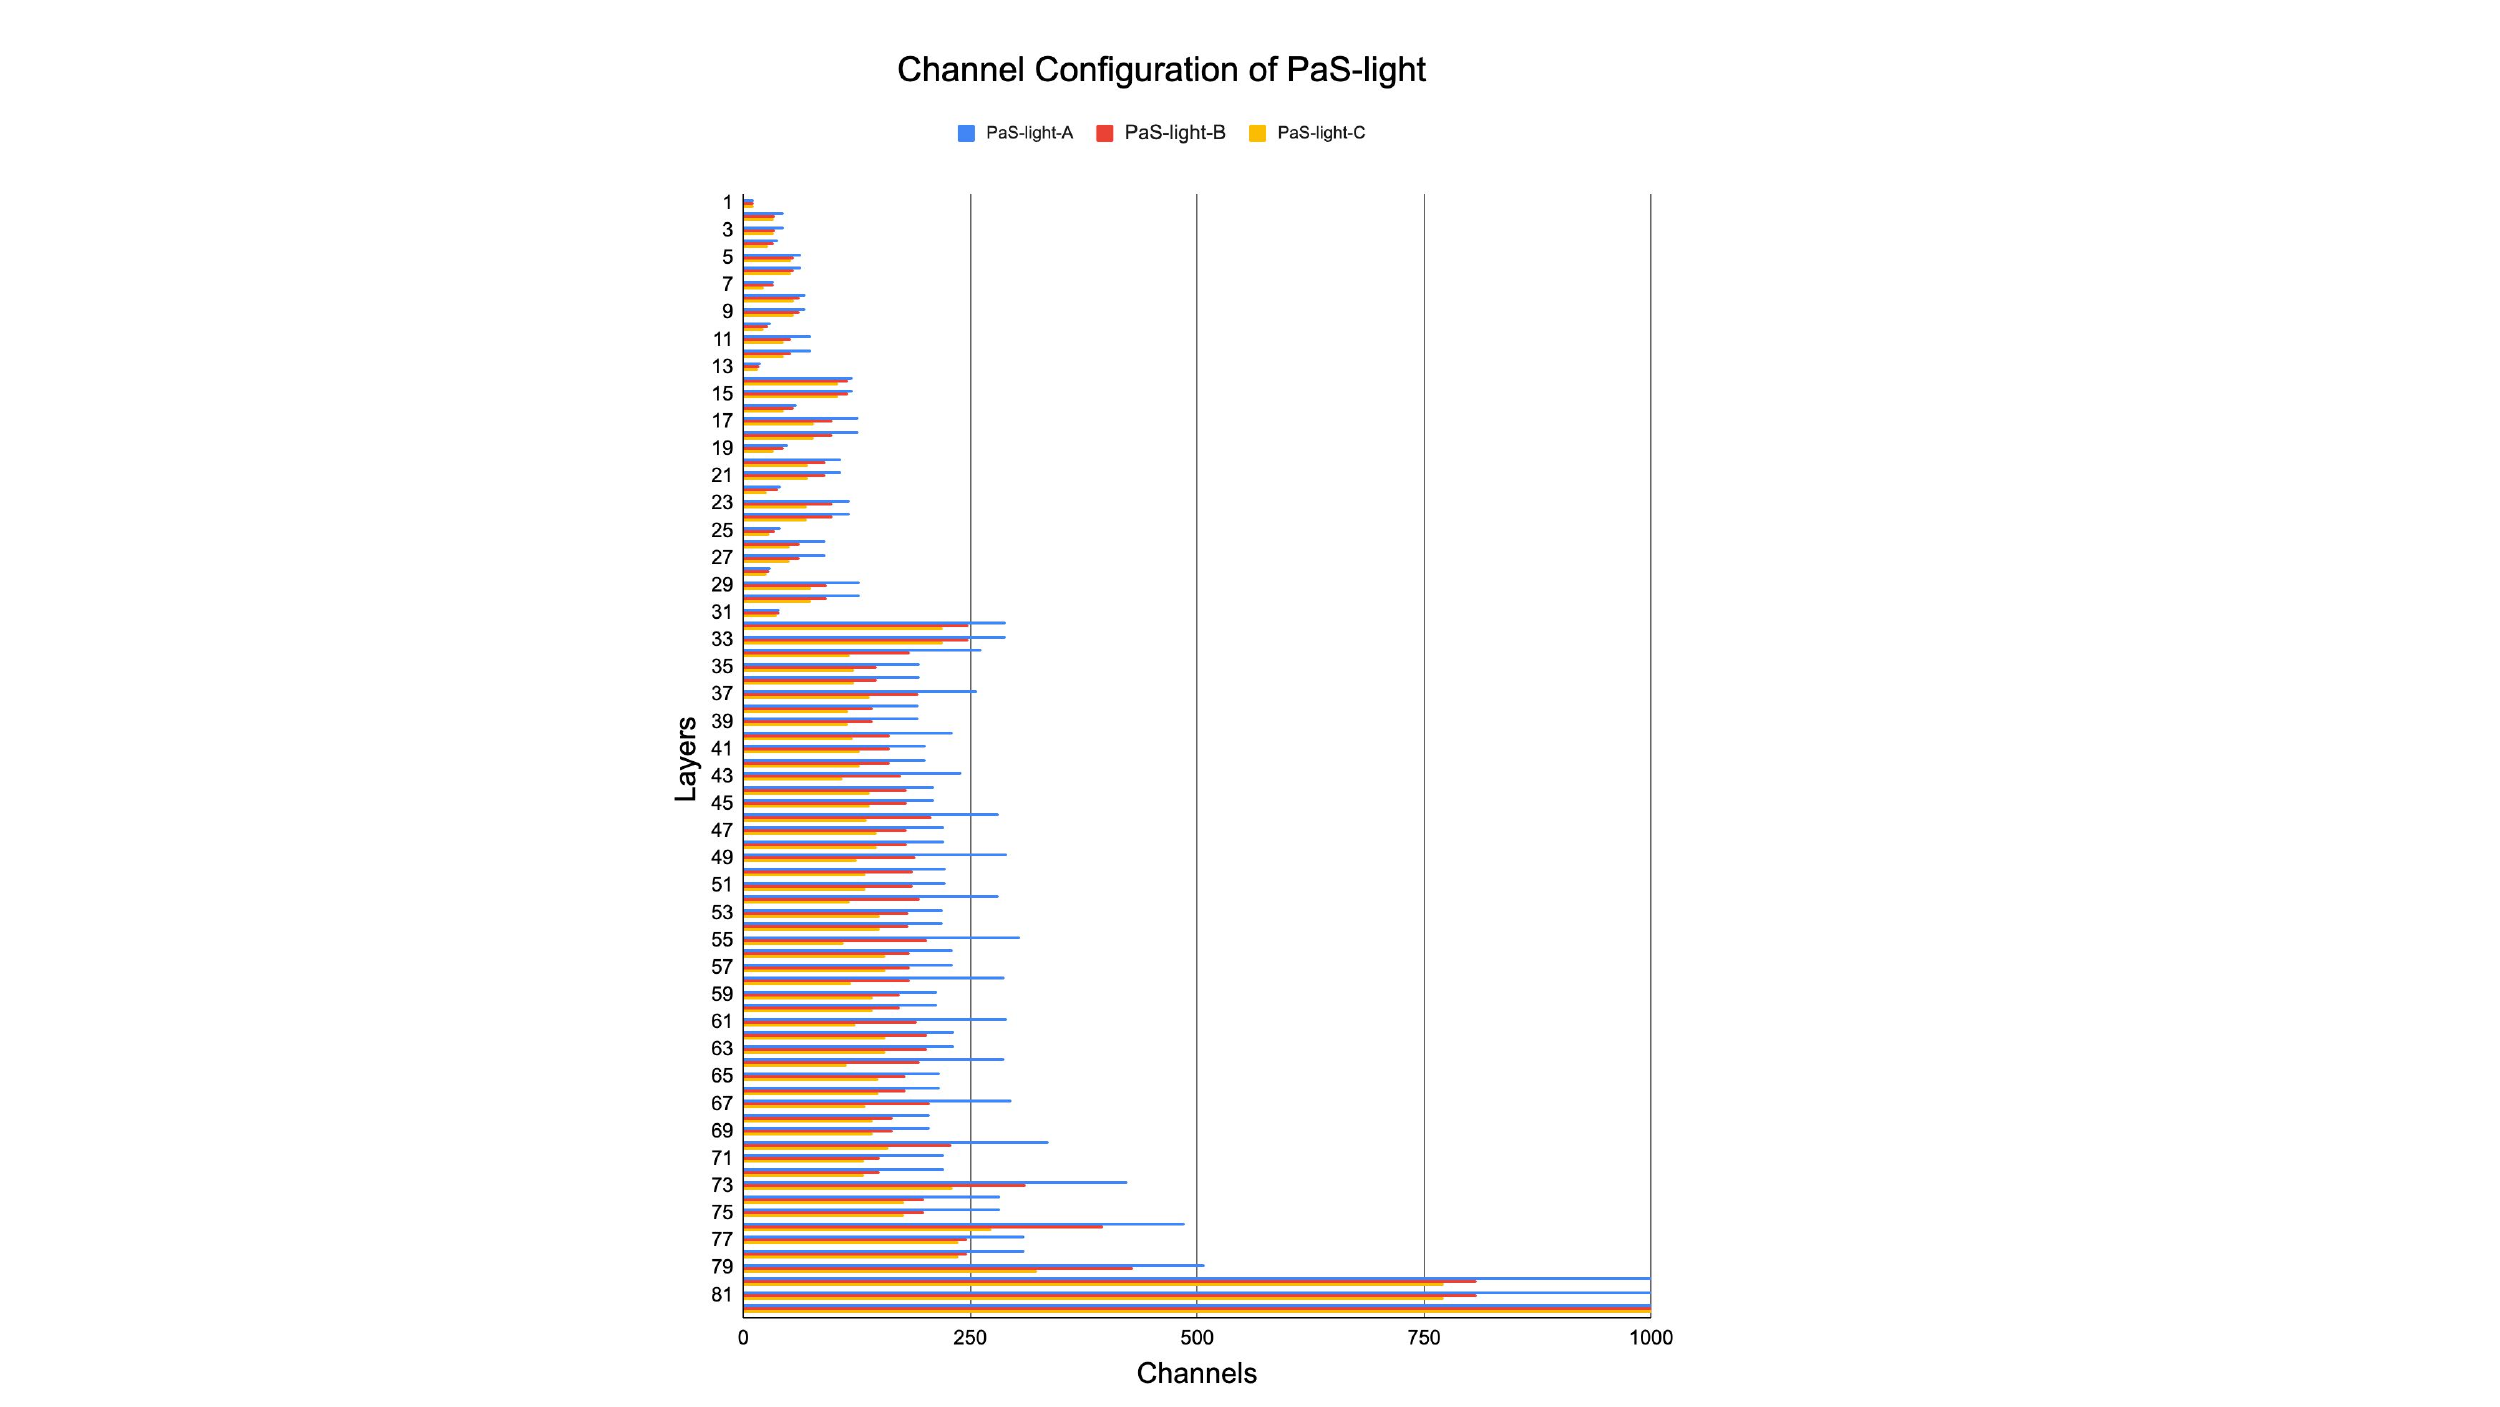}
  \caption{A series of PaS searched channel configurations for lightweight backbone. }
  \label{fig:appendixlight}
\end{figure}

\begin{figure}[]
  \small
  \centering
  \includegraphics[width=0.9\columnwidth]{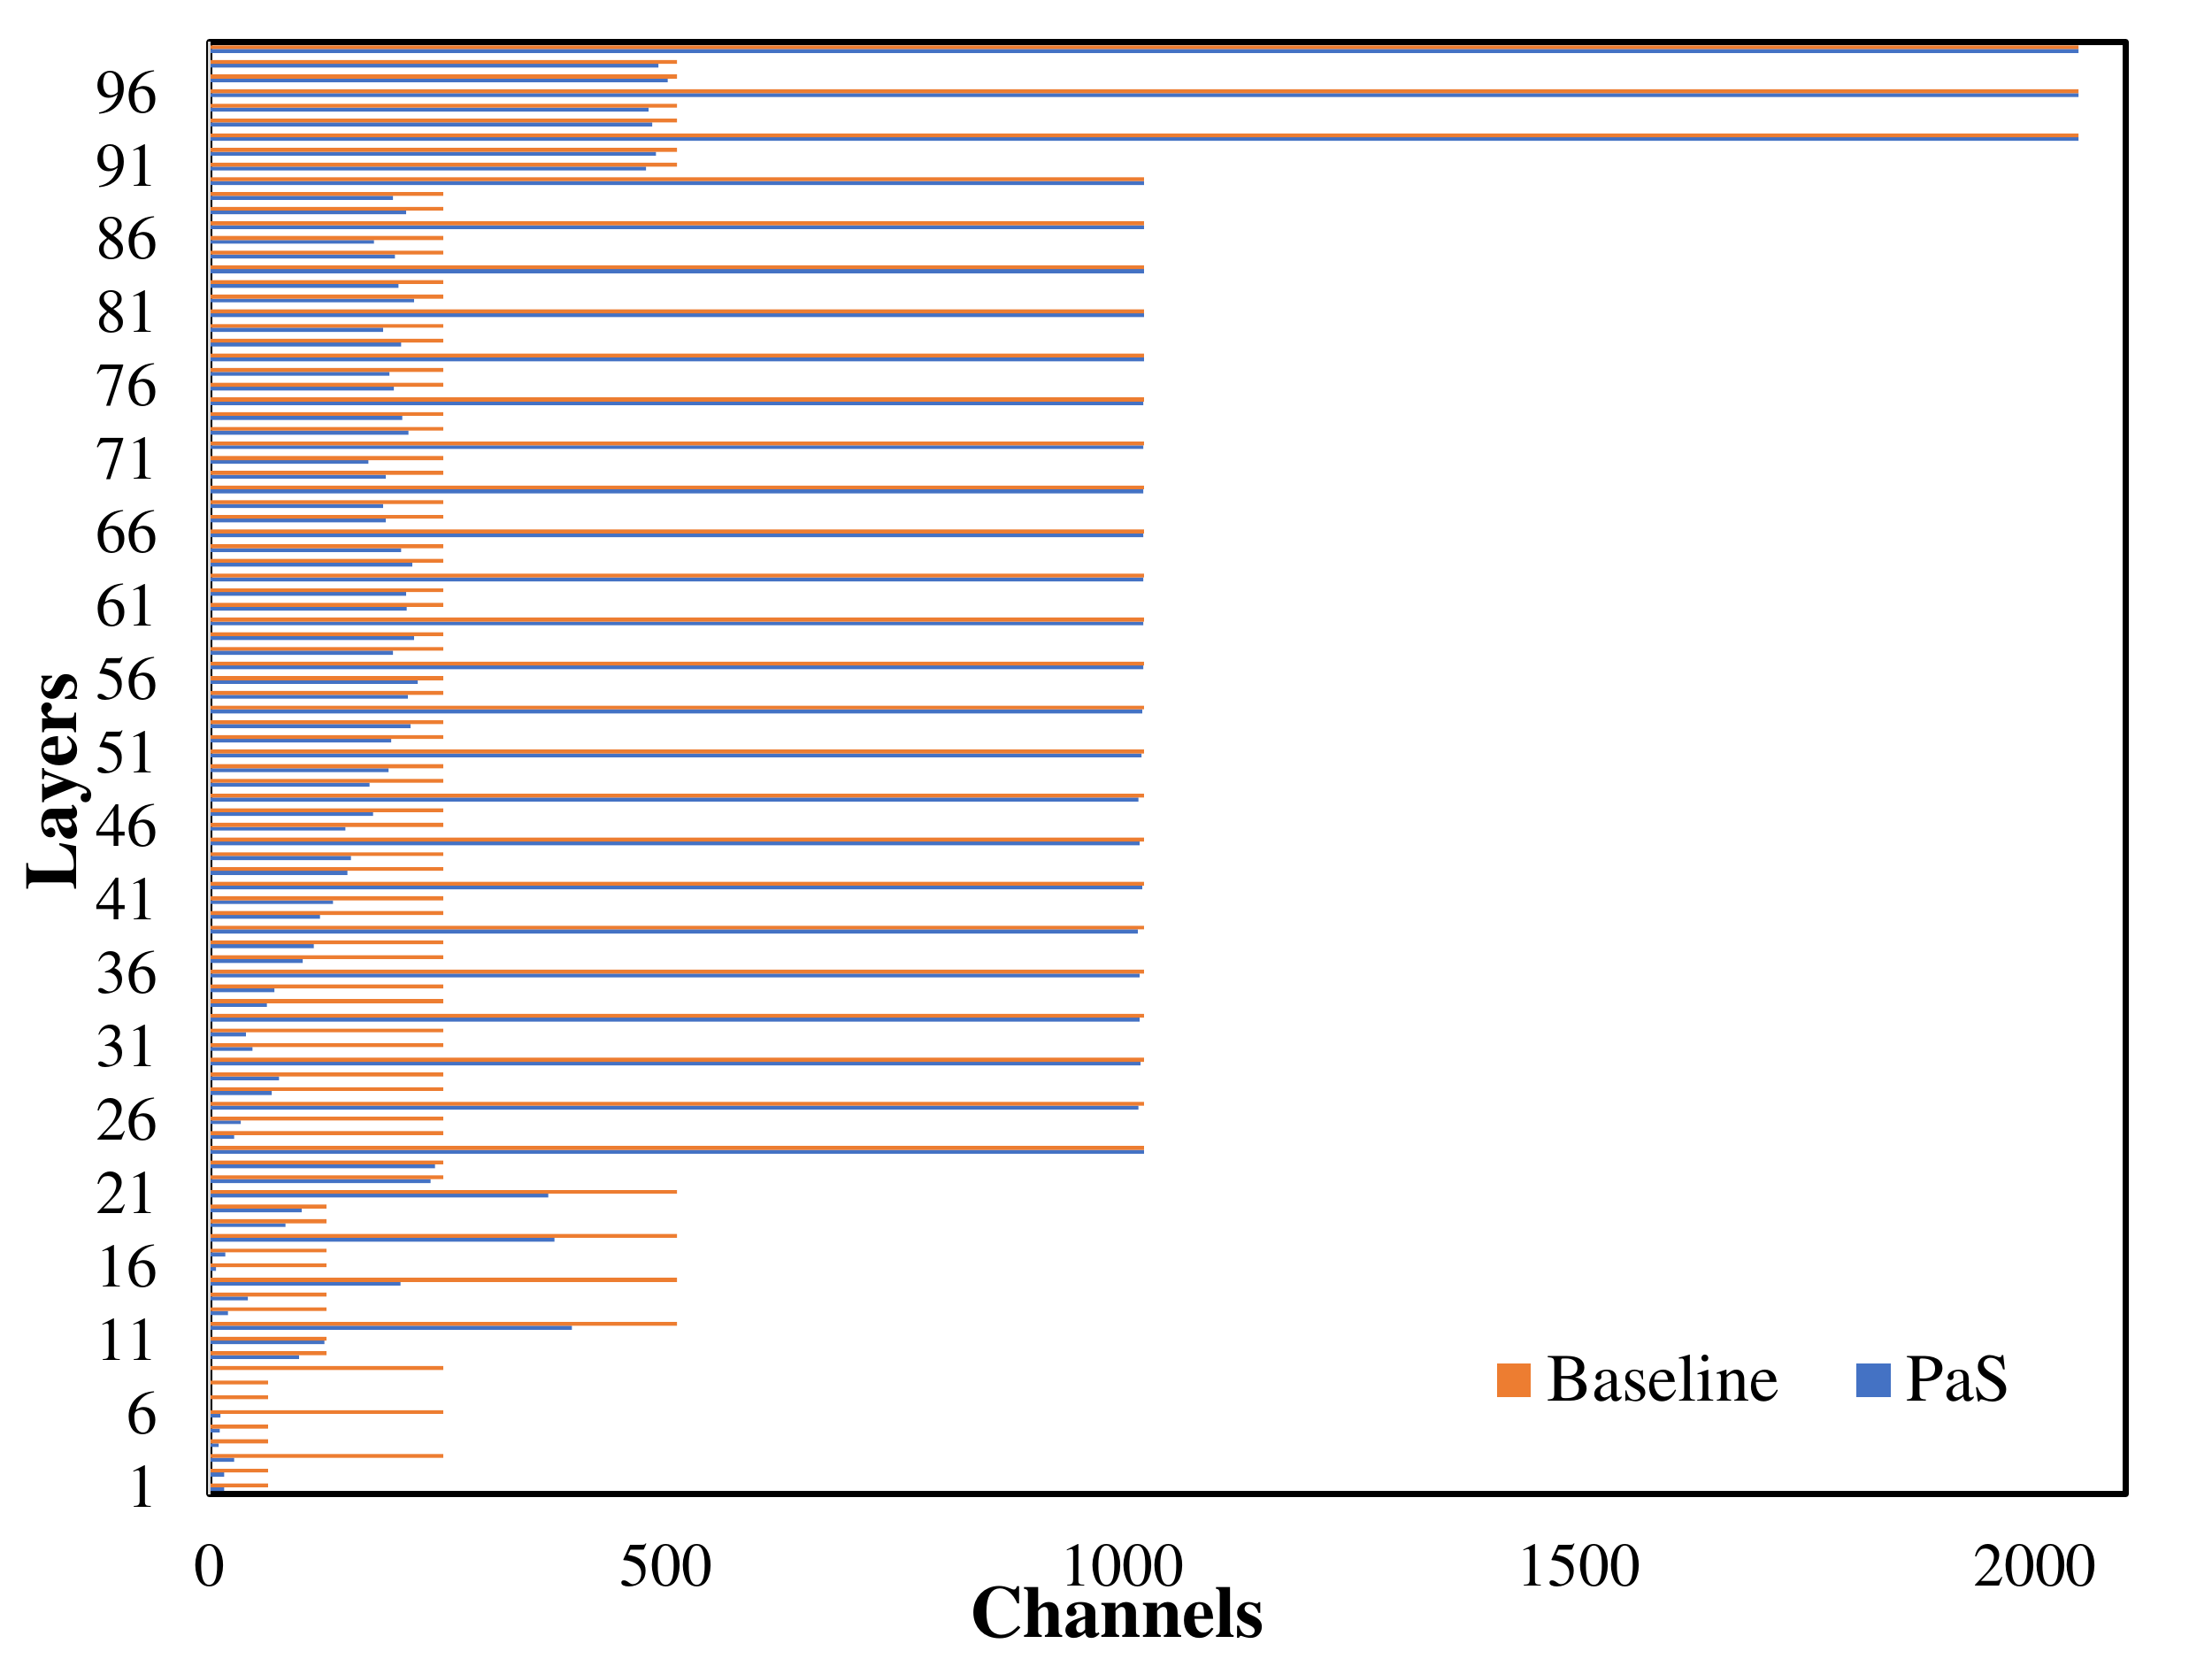}
  \caption{YOLACT channel configuration searched by PaS, with ResNet101 backbone, compressing $1.7\times$ GMACs. }
  \label{fig:appendixc}
\end{figure}

\begin{figure}[]
  \small
  \centering
  \includegraphics[width=0.9\columnwidth]{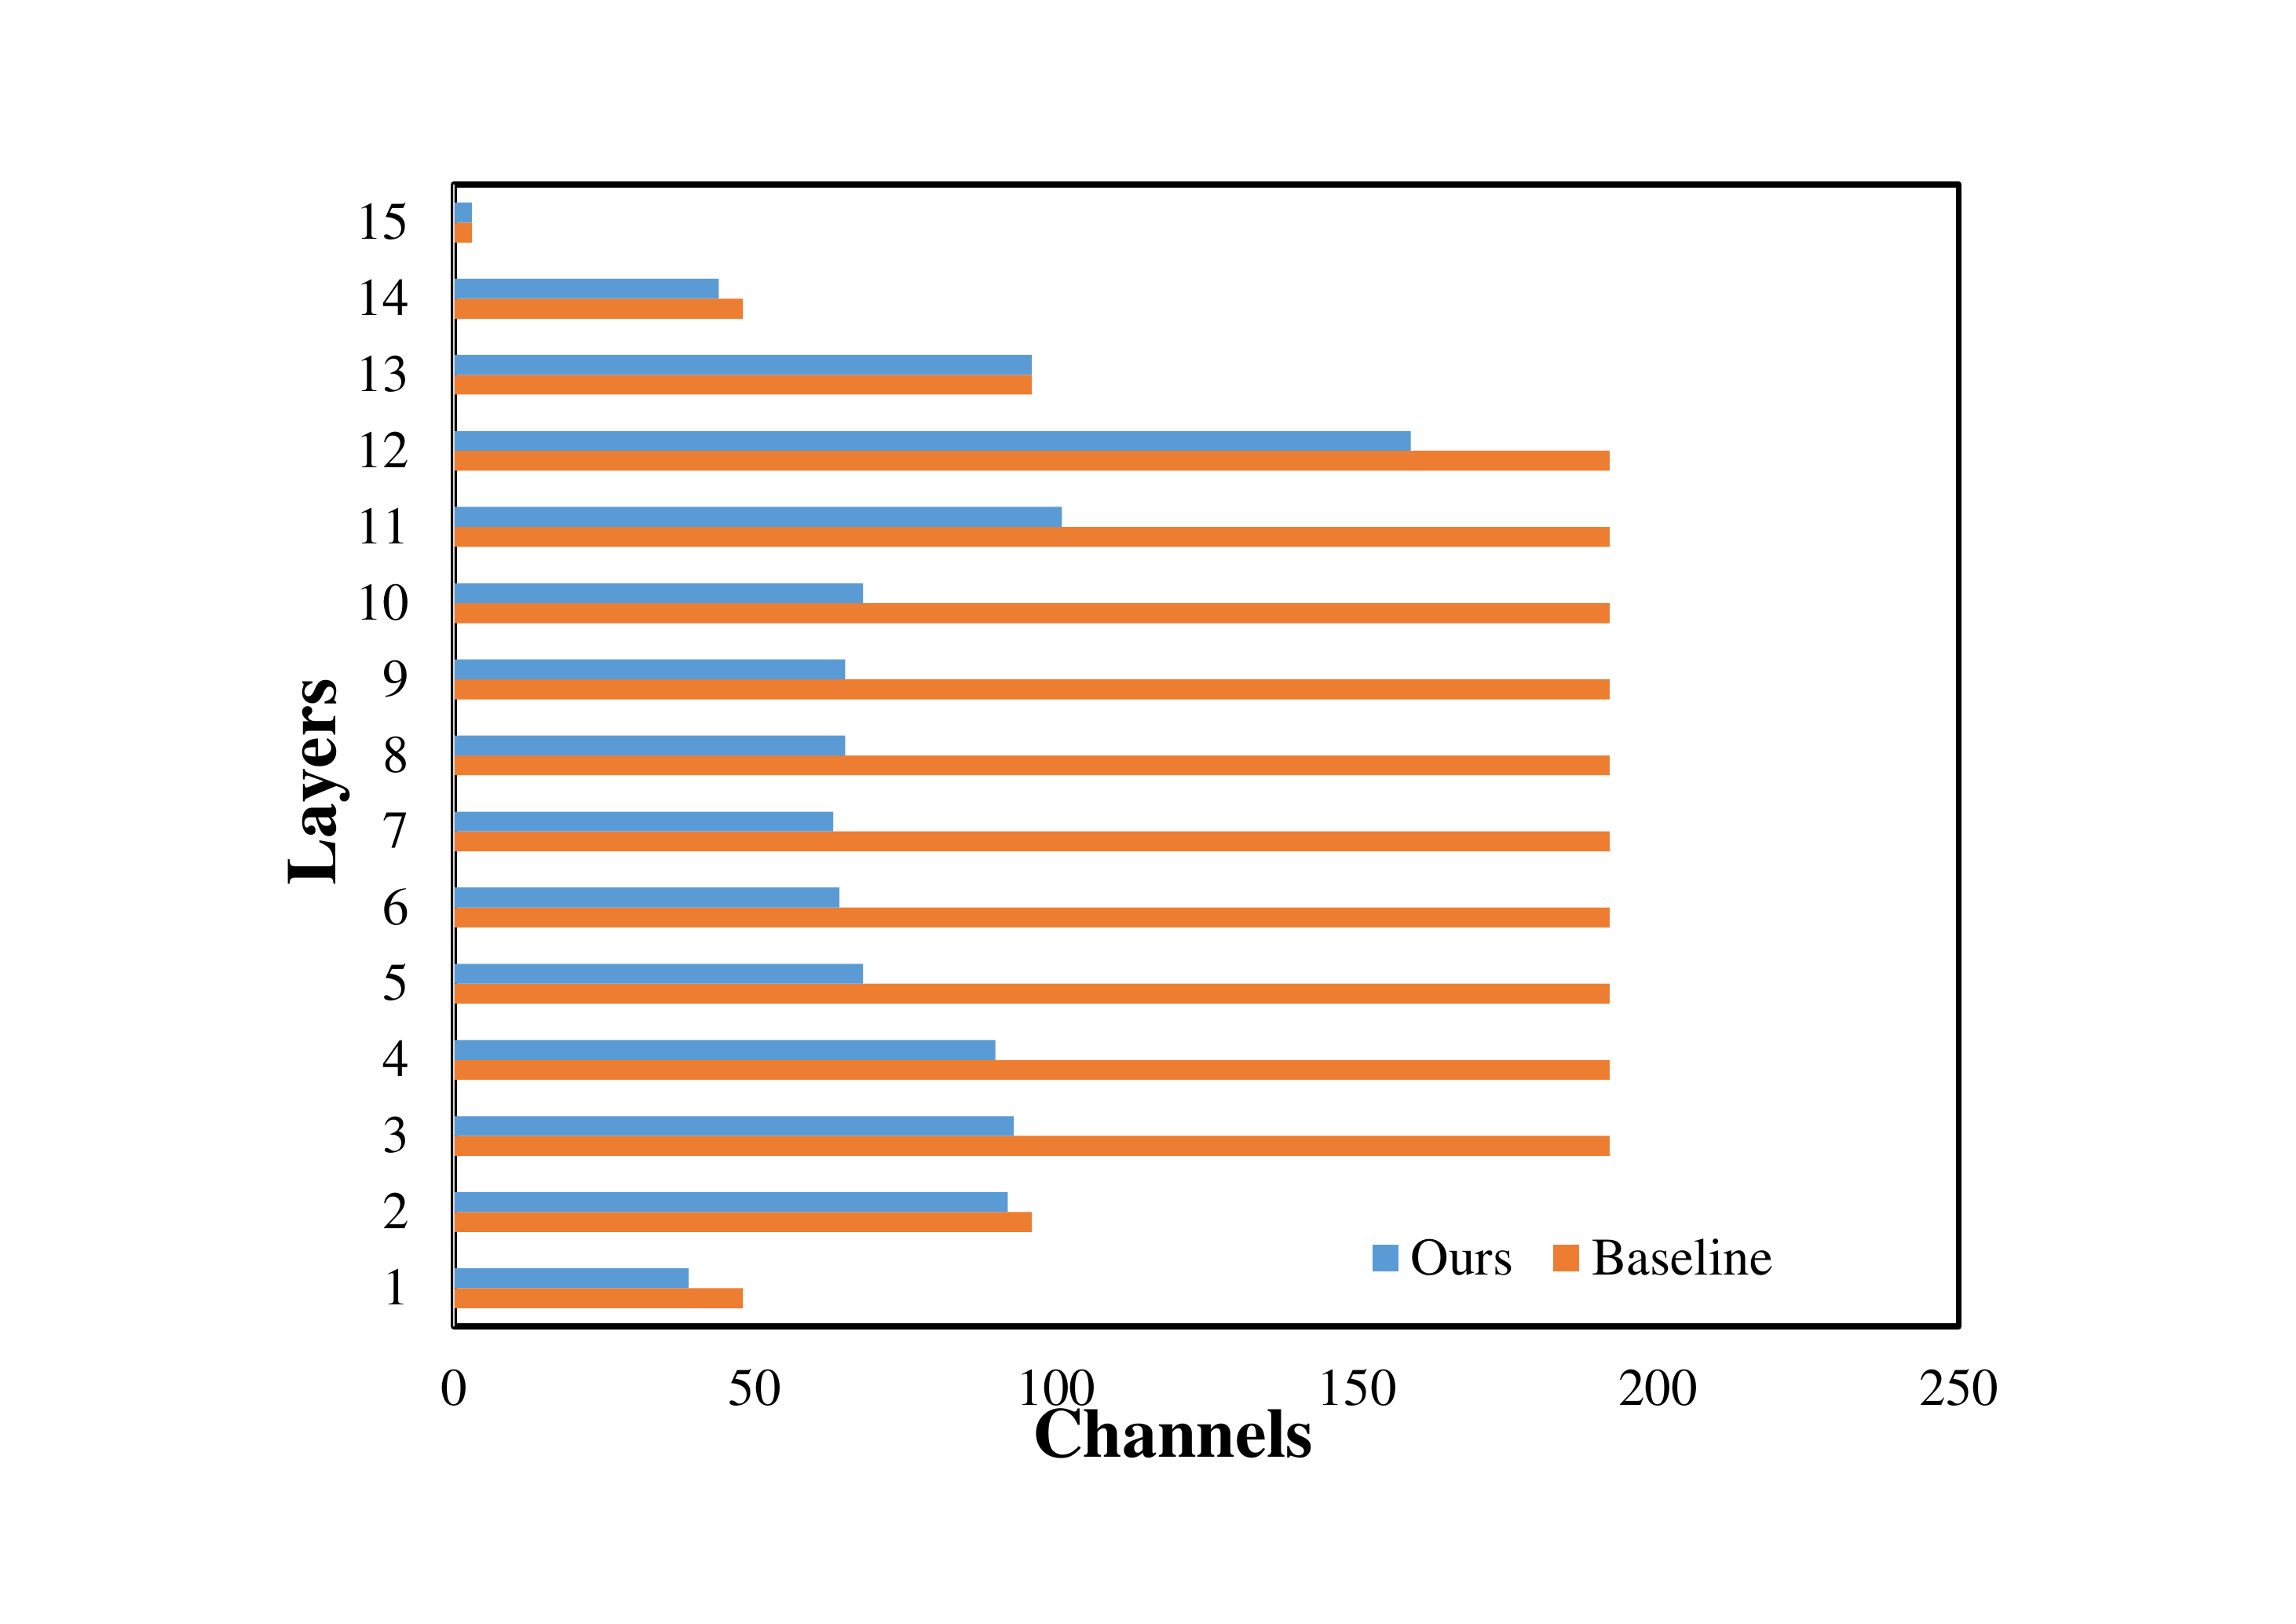}
  \caption{CycleGAN channel configuration searched by PaS, compressing to 2.7 GMACs. Note that the width of mobile-ResNet backbone layers is decided by block. }
  \label{fig:appendixd}
\end{figure}

% \subsection{MobileNet-V2} \label{app: MobileNet-V2}

% We also demonstrate the power of PaS on light weight MobileNet-V2 model as shown in Tab.~\ref{tab:mobilenet}. 
% MobileNet-V2~\cite{sandler2018mobilenetv2} is a stack of inverted residual block which contains 3 convolution layers $\{1\times1, 3\times3, 1\times 1\}$, where the middle $3\times 3$ one is depth-wise convolution to reduce computation complexity. 
% We choose MobileNet-V2 $1.3\times$ as the pruning super-net, which is 504 MMACs with $74.2\%$ top-1 accuracy. 
% We compare our PaS with other search or pruning methods targeting on approximately 210 MMACs and 150 MMACs, and demonstrate that our PaS consistently outperforms current arts. 

% \begin{table}[b!]
% \small
% \centering
% \caption{MobileNet-V2 model on ImageNet dataset.}
% \begin{tabular}{c|ccc}
% \toprule
% Method       & MMACs        & Top1          & Top5          \\
% Baseline     & 311          & 71.2          & 90.3          \\
% \hline
% MetaPruning  & 217          & 71.2          &    /           \\
% LEGR         & 210          & 71.4          &     /          \\
% AMC          & 220          & 70.9          &     /          \\
% \textbf{PaS} & \textbf{217} & \textbf{71.5} & \textbf{90.3} \\
% \hline
% AMC          & 150          & 70.8          &      /         \\
% TAS          & 150          & 70.9          &      /         \\
% \textbf{PaS} & \textbf{150} & \textbf{71.0} & \textbf{90.1} \\
% \bottomrule
% \end{tabular}
% \label{tab:mobilenet}
% \end{table}

\subsection{Experiment Details for YoLACT and GAN} \label{app: gan}  
To validate the effectiveness of PaS, we conduct extensive experiments on large scale and complex tasks including instance segmentation and image to image translation by Generative Adversarial Networks (GAN). 
In this section we provide experiment details of the aforementioned tasks for easy replication. 
Codes and models will be available upon publication.

\textbf{YOLACT}~\cite{bolya2019yolact} %is a GPU real time instance segmentation model. 
can achieve real-time instance segmentation on GPU. 
We set input resolution to $550\times 550$, leveraging ResNet101 with weights pretrained on ImageNet-1000 as backbone. 
Following origin settings, we initialize learning rate at $10^{-3}$ and decayed by $10^{-1}$ at selected iterations. 
Compared to origin implementation trained with batch size 8, we use a larger batch size of 64 over 8 NVIDIA RTX TITAN GPUS and scale initial learning rate proportionally by $8\times$, while reducing origin iterations from 80k to 10k. 
The model is trained with SGD and momentum is set to be 0.9. 

\textbf{GAN} is widely recognized as difficult to train because of unstable convergence and mode collapse. 
Currently very few work can directly perform search or automatic pruning on GAN tasks. 
We conduct experiments on CycleGAN~\cite{zhu2020unpaired} which performs un-paired image to image translation. 
We adopt the mobile resnet architecture in \cite{li2020gan} with width multiplier 64 as pruning super-net, and train with batch size 32 over 8 NVIDIA GeForce RTX 2080Ti GPUs. 
Learning rate is set to $2\times 10^{-4}$ for both generator and discriminator, with ADAM optimizer and LSGAN loss. 
Leaning rate is fixed for the first 400 epochs and then linearly decayed to zero in 600 epochs.
We choose instance normalization without tracking running statistics as it achieves best performance. 
Note that only the generator is used at inference stage to generate target images, thus our PaS is not applied to discriminator. 

Generative quality of our PaS model compared to~\cite{li2020gan} on horse to zebra image translation benchmark, with CycleGAN~\cite{zhu2020unpaired} method. 

\begin{figure*}[b!]
  \small
  \centering
  \includegraphics[width=1.2\columnwidth]{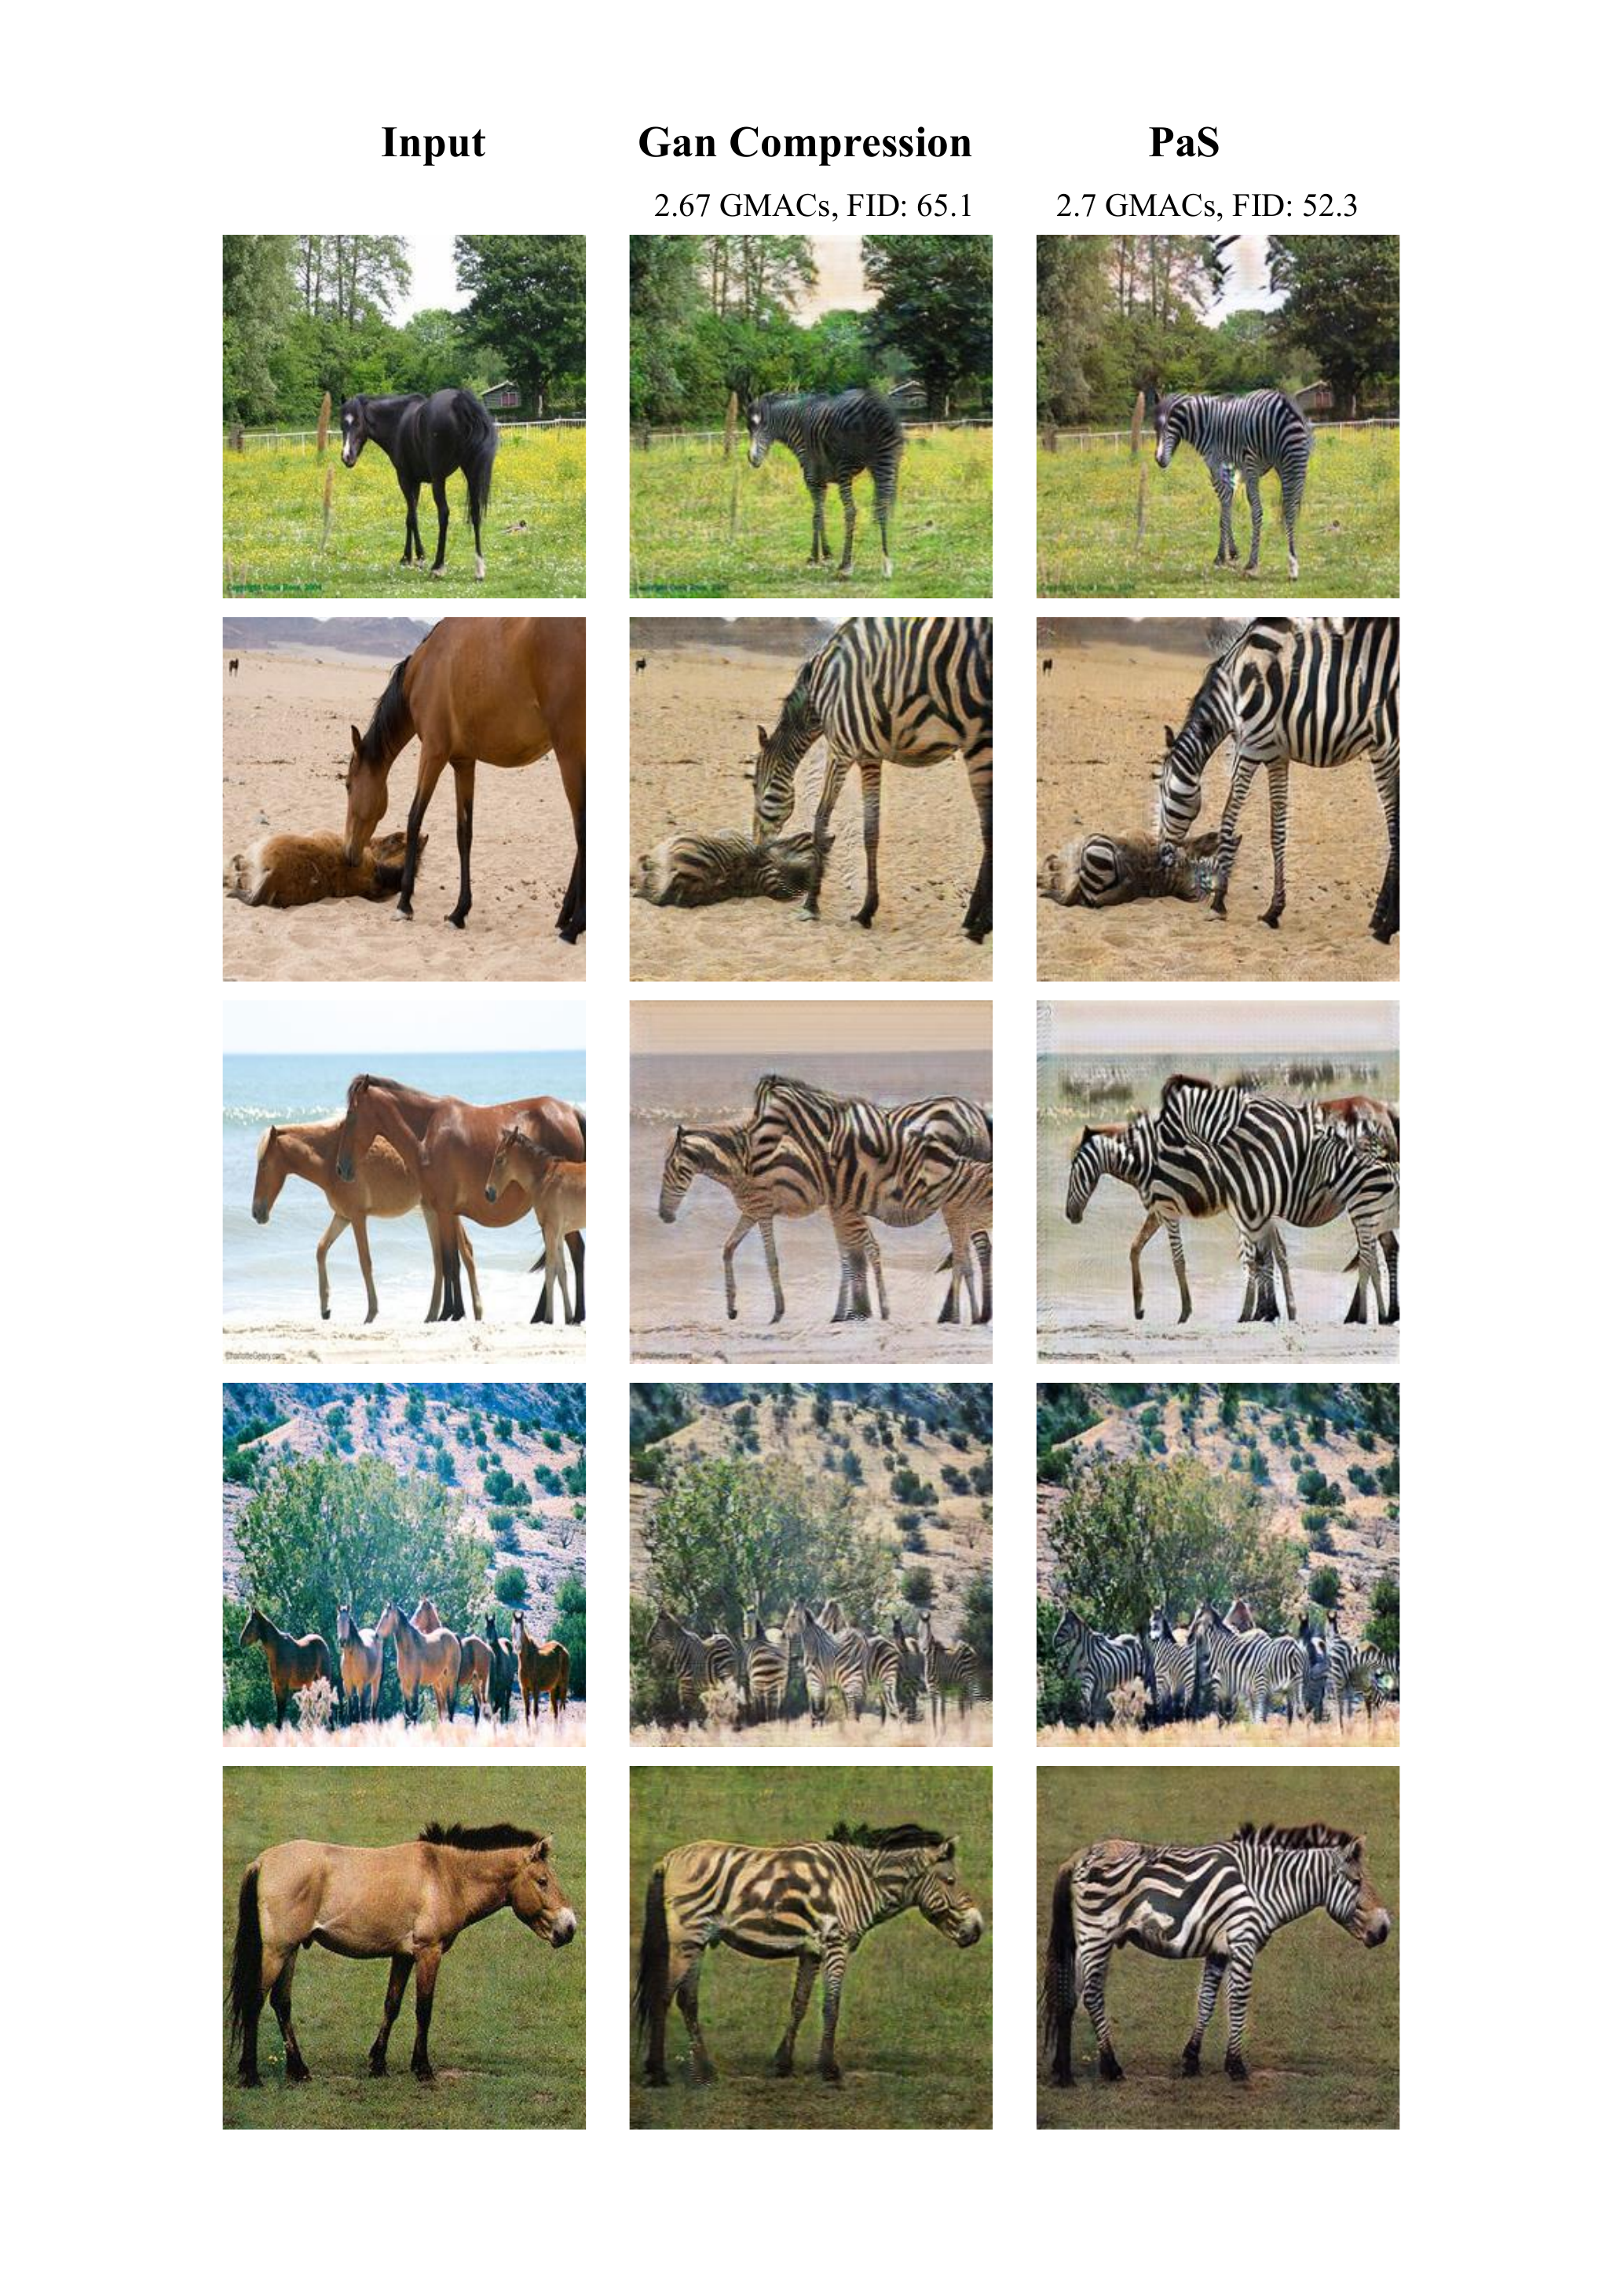}
  \caption{Generative quality of our PaS model on horse to zebra image translation benchmark.}
  \label{fig:appendixe}
\end{figure*}

\begin{figure*}[b!]
  \small
  \centering
  \includegraphics[width=1.6\columnwidth]{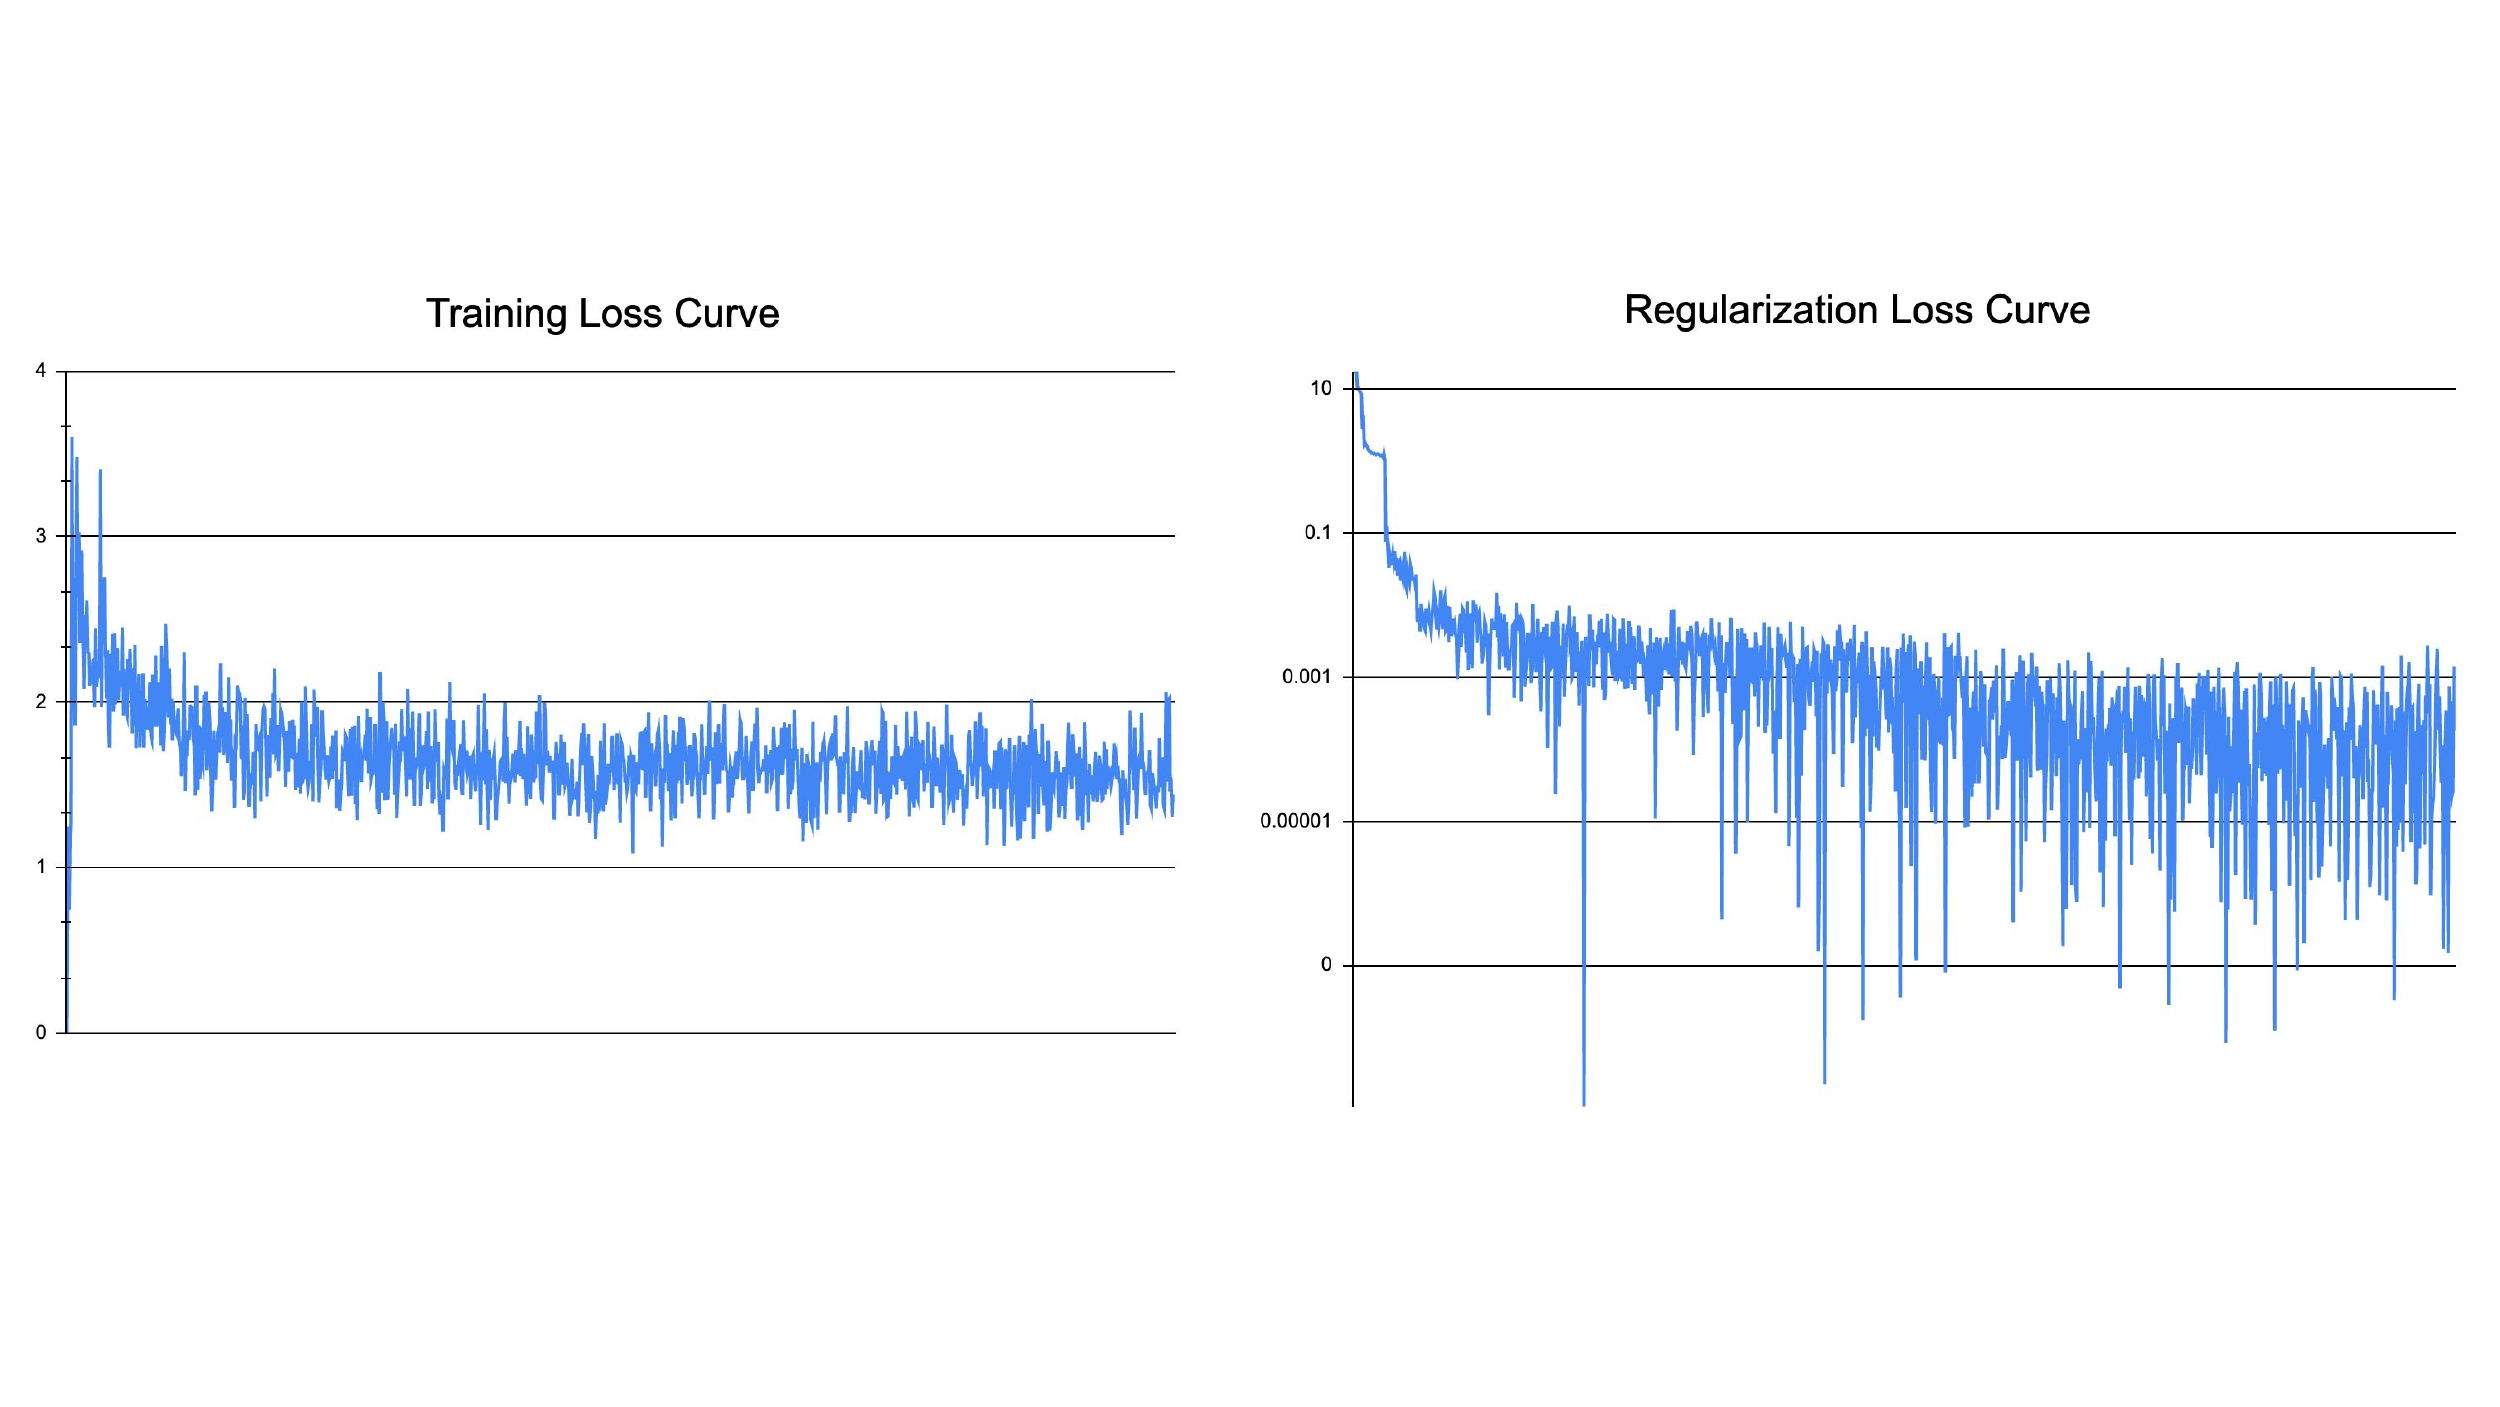}
  \caption{An example loss curve of PaS-C. We can oberve that the regularization loss continue to decrease and converge very close to zero, proving that the final policy satisfies the resource constraint. The origin training loss slightly diverges when the searching starts due to pruned channels, but is able to recover after the network adapts to pruning. We can also observe strong vibration in regularization loss, which is a desired phenomenon implying exploration. }
  \label{fig:appendix_loss}
\end{figure*}
